# Supplementary material for: Understanding the Impact of Referent Design on Scale Perception in Immersive Data Visualization
Source: arXiv:2403.16018 source file (2024-03-24)
Supplement: Supplementary file 1 [file 7_Appendix.tex]

\appendix
% \section{Appendix}
% \begin{figure}[htb]
%     \centering
%     \includegraphics[width=0.95\linewidth]{Figures/Stimuli.pdf}
%     \caption{Stimuli used in the experiment.}
%     \label{fig:result-significants}
% \end{figure}
% \section{Appendix2}
